# Supplementary material for: A Reinforcement Learning Framework for Dynamic Mediation Analysis
Source: arXiv:2301.13348 source file (2023-09-03)
Supplement: Supplementary file 1 [file 9_Appendix.tex]

\section{Others for non-parametric}
\textbf{Objective.} \begin{equation}
    argmin_{\eta^{\pi_e},Q^{\pi_e}}T^{-1}\sum_{t=1}^{T}\big[R+ \Mean_{\substack{a\sim \pi_e(\bullet|S')\\ m\sim p(\bullet|a,S')}} Q^{\pi_e}(S',a,m)-\Mean_{m\sim p(\bullet|A,S)}Q^{\pi_e}(S,A,m)\big]^{2}-\eta^{\pi_e}
\end{equation}

\textbf{Coupled Estimation.} 
\begin{equation}
    argmin_{\eta^{\pi_e},Q^{\pi_e}}T^{-1}\sum_{t=1}^{T}\hat{g}_{i}^{2}(A_t,S_t,M_t;\eta^{\pi_e},Q^{\pi_e})+\lambda\|Q^{\pi_e}\|^{2},
\end{equation}where
\begin{multline}
    \hat{g} = argmin_{g}T^{-1}\sum_{t=1}^{T}\big[R+ \Mean_{\substack{a\sim \pi_e(\bullet|S')\\ m\sim p(\bullet|a,S')}} Q^{\pi_e}(S',a,m)-\Mean_{m\sim p(\bullet|A,S)}Q^{\pi_e}(S,A,m)-\eta^{\pi_e}\\
    -g(A_{t},S_{t},M_{t})\big]^{2}+\mu\|g\|^{2},
\end{multline}
Considering the class of linear regression, let 
\begin{align}
    g(A_{t},S_{t},M_{t}) & = [1,S_t,A_t,M_t]\beta = \boldsymbol{z}_t\beta \\
    Q^{\pi_e}(S_t,A_t,M_t) & = [S_t, A_t, M_t]\theta =\tilde{\boldsymbol{z}_t}\theta.
\end{align}
Therefore, we can rewrite the $\hat{g}$ as
\begin{multline}
    argmin_{\beta}\frac{1}{NT}\sum_{i,t}\Big\{R_{i,t}+\Mean_{\substack{a\sim \pi_e(\bullet|S')\\ m\sim p(\bullet|a,S')}} Q^{\pi_e}(S',a,m)-\Mean_{m\sim p(\bullet|A,S)}Q^{\pi_e}(S,A,m)
    -\eta^{\pi_e}-\boldsymbol{z}_{i,t}\beta\Big\}^{2}+\mu\beta^{T}\beta.
\end{multline} The closed form expression of $\beta$ is 
\begin{align}
    \hat{\beta} = (\boldsymbol{Z}^{T}\boldsymbol{Z}+NT\mu\boldsymbol{I}_{p})^{-1}\boldsymbol{Z}^{T}(\boldsymbol{R}+\boldsymbol{Q}^{(2)}-\eta^{\pi_e}\boldsymbol{1}-\boldsymbol{Q}^{(1)}).
\end{align}
Then $\hat{g}(S_t,A_t,M_t) = \boldsymbol{z}_t\hat{\beta}$, and 
\begin{align}
    \frac{1}{NT}\sum_{i,t}\hat{g}^{2}(A_{i,t},S_{i,t},M_{i,t};\eta^{\pi_e},Q^{\pi_e}) = \frac{1}{NT} \beta^{T}\boldsymbol{Z}^{T}\boldsymbol{Z}\beta.
\end{align}
With $Q^{\pi_e}(S_t,A_t,M_t) = [S_t, A_t, M_t]\theta =\tilde{\boldsymbol{z}_t}\theta$, we have that
\begin{align*}
    \Mean_{m\sim p(\bullet|A,S)}Q^{\pi_e}(S,A,m) &= [S,A,\Mean(m|A,S)]\theta = \boldsymbol{\tilde{z}_{i,t}^{(1)}}\theta\\
    \Mean_{\substack{a\sim \pi_e(\bullet|S')\\ m\sim p(\bullet|a,S')}} Q^{\pi_e}(S',a,m) &= [S',\Mean^{\pi_{e}}(a|S'),\Mean^{\pi_e}(m|S')]\theta = \boldsymbol{\tilde{z}_{i,t}^{(2)}}\theta.
\end{align*} Therefore, 
\begin{align*}
    \Mean_{\substack{a\sim \pi_e(\bullet|S')\\ m\sim p(\bullet|a,S')}} Q^{\pi_e}(S',a,m)-\Mean_{m\sim p(\bullet|A,S)}Q^{\pi_e}(S,A,m) = (\boldsymbol{\tilde{z}_{i,t}^{(2)}}-\boldsymbol{\tilde{z}_{i,t}^{(1)}})\theta = \boldsymbol{\tilde{z}_{i,t}}\theta
\end{align*}
Let 
\begin{align*}
    \boldsymbol{G} = \boldsymbol{Z}(\boldsymbol{Z}^{T}\boldsymbol{Z}+NT\mu\boldsymbol{I}_{p})^{-1}\boldsymbol{Z}^{T}\boldsymbol{Z}(\boldsymbol{Z}^{T}\boldsymbol{Z}+NT\mu\boldsymbol{I}_{p})^{-1}\boldsymbol{Z}^{T},
\end{align*} and
\begin{align*}
    \alpha = [\theta^{T},\eta^{\pi_e}]^{T}.
\end{align*}
\begin{align}
    \hat{\alpha} = argmin_{\alpha} \frac{1}{NT}[\boldsymbol{R}+[\boldsymbol{\tilde{Z}}, -\boldsymbol{1}]\alpha]^{T}\boldsymbol{G}[\boldsymbol{R}+[\boldsymbol{\tilde{Z}}, -\boldsymbol{1}]\alpha]+\frac{1}{NT}\alpha^{T}\begin{bmatrix}
NT\lambda \boldsymbol{I}_p & \boldsymbol{0}\\
0 & 0
\end{bmatrix}\alpha.
\end{align}
The closed form expression of $\hat{\alpha}$ is then,
\begin{align}
    \hat{\alpha} = \Big\{[\boldsymbol{\tilde{Z}}, -\boldsymbol{1}]^{T}\boldsymbol{G}[\boldsymbol{\tilde{Z}}, -\boldsymbol{1}] + \begin{bmatrix}
NT\lambda \boldsymbol{I}_p & \boldsymbol{0}\\
0 & 0
\end{bmatrix}\Big\}^{-1}[\boldsymbol{\tilde{Z}}, -\boldsymbol{1}]^{T}\boldsymbol{G}\boldsymbol{R}
\end{align}

Binary A, the simplest linear regression. CV is required to decide the tuning parameter.

%fitted Q-evaluation Method \citep{le2019batch}, it can be showed that the Q-estimate is consistent \citep{fan2020theoretical}

%estimate the $\omega$ by solving the equation $L$
