# Supplementary material for: A Reinforcement Learning Framework for Dynamic Mediation Analysis
Source: arXiv:2301.13348 source file (2023-09-03)
Supplement: Supplementary file 2 [file Potential_Outcome.tex]

\section{Potential Outcome (Version 1)}
%where $\Mean^{\pi}$ denotes the expectation by assuming that %the treatment $a$ is repeatedly assigned all the time. 
%the system follows a given stationary policy $\pi$ and $a_0$ denotes a nondynamic policy that assigns a fixed treatment $a_0$ all the time. 

%\begin{eqnarray*}
%	&&\textrm{ATE}=\Mean \omega^{\pi_e}(S_t) \frac{\pi_e(A_t|S_t)}{\pi_b(A_t|S_t)}R_t-\Mean \omega^{a_0}(S_t) \frac{\mathbb{I}(A_t=a_0)}{\pi_b(A_t|S_t)}R_t\\
%	&=&\sum_m \Mean \left[ \omega^{\pi_e}(S_t) \frac{\pi_e(A_t|S_t)}{\pi_b(A_t|S_t)}-\omega^{a_0}(S_t) \frac{\mathbb{I}(A_t=a_0)}{\pi_b(A_t|S_t)} \right] r(S_t,A_t,m)p_m(m|S_t,A_t)\\
%	&=&\sum_{a,m} \Mean[\pi_e(a|S_t)\omega^{\pi_e}(S_t) r(S_t,a,m)p_m(m|S_t,a) -\pi_0(a|S_t)\omega^{a_0}(S_t) r(S_t,a,m)p_m(m|S_t,a)]
%\end{eqnarray*}
%where $\omega^{\pi}$ denotes , %the policy that repeatedly assigns $a$ and that under the behavior policy, 

%By definition, ATE can be decomposed into three terms: direct effect of the treatment(DE), indirect effect of mediator(ME), and indirect effect of the state (SE). Specifically,
%\begin{equation}
%   ATE = DE+ME+SE.
%\end{equation}

We first start with some notations. For any variable $W$, let $\bar{W}_t = (W_0, W_1,\cdots, W_t)$ denote the history of $W$, and $H_t=(\bar{S}_t,\bar{A}_t,\bar{M}_t)$ be the history of all variables, until step $t$. By convention, $\bar{W}_t = \emptyset$ if $t < 0$. Analogously, we use $\bar{W}_t^{\pi} = (W_0^{\pi}, W_1^{\pi},\cdots, W_t^{\pi})$ to denote the history of $W$ if policy $\pi$ were followed, and $H^{\pi}_t=(\bar{S}_t^{\pi},\bar{A}_t^{\pi},\bar{M}_t^{\pi})$. Let $\pi(s)$ denote the action would be taken by the policy $\pi$ if we observed state $s$, then we use $\bar{d}_{1,\bar{s}_1}^{\pi} =(\pi(s_0),\pi\{\bar{s}_1,\pi(s_0)\})$ to denote the actions would be taken at first two steps under policy $\pi$ and conditional on $\bar{s}_1$. Recursively, we use $\bar{d}_{t,\bar{s}_t}^{\pi} = (\pi(s_0), \pi\{\bar{s}_1, \pi(s_0)\}, \cdots,  \pi\{\bar{s}_t, \bar{d}_{t-1,\bar{s}_{t-1}}^{\pi}\})$ to denote the action sequence would be selected through step $t$ for $t>1$, following policy $\pi$, given the state sequence $\bar{s}_t$. Similarly, conditional on $\bar{s}_t$, let $\bar{M}_{t,\bar{s}_t}(\bar{d}^{\pi}_{t,\bar{s}_t})$ denotes the values of the mediator that would have been observed if the actions $\bar{d}^{\pi}_{t,\bar{s}_t}$ has been taken sequentially, and $R_{t,\bar{s}_t}(\bar{d}^{\pi_1}_{t,\bar{s_t}},\bar{M}_{t,\bar{s}_t}(\bar{d}^{\pi_2}_{t,\bar{s_t}}))$ be the potential reward that would be observed if the action sequence $\bar{A}_t$ is set to $\bar{d}^{\pi_1}_{t,\bar{s_t}}$ and the mediator sequence $\bar{M}_t$ is set to $\bar{M}_{t,\bar{s}_t}(\bar{d}^{\pi_2}_{t,\bar{s_t}})$. 

\textbf{Alternative Definition of action sequence:}
For any policy $\pi$, denote $\bar{d}_{t,\bar{s}_t}^{\pi} = \{d_k^{\pi}(\cdot)\}_{0\leq k \leq t}$ a sequence of independent, $\mathcal{A}$-valued stochastic process depend on the state sequence $\bar{s}_t^{\pi}$, where $P\{d_k^{\pi}(s_{k}) = a_k\} = \pi(a_k|s_k)$.

In the rest of the paper, for the sake of brevity, we omit the subscript $\bar{s}_t$ and use $\bar{d}^{\pi_1}_t$, $\bar{M}_{t}(\bar{d}^{\pi_2}_t)$, and $R_t(\bar{d}^{\pi_1}_t,\bar{M}_{t}(\bar{d}^{\pi_2}_t))$ to denote the counterfactual information conditional on some state information $\bar{S}^{\pi}_t$ as the equation implies. For example, $\Mean^{\pi_1}[R_t(\bar{d}^{\pi_2}_t,\bar{M}_{t}(\bar{d}^{\pi_3}_t))]$ implies that the $\bar{d}^{\pi_2}_t$, $\bar{M}_{t}(\bar{d}^{\pi_3}_t)$, and $R_t(\bar{d}^{\pi_1}_t,\bar{M}_{t}(\bar{d}^{\pi_2}_t))$ are conditional on the potential state sequence $\bar{S}^{\pi_1}_t$ that would be observed if policy $\pi_1$ were followed. Mathematically, $\bar{S}^{\pi_1}_t = (S_0,S_1^{\pi_1}(H^{\pi_1}_{0}),\cdots,S_t^{\pi_1}(H^{\pi_1}_{t-1}))$, where $S_t^{\pi_1}(H^{\pi_1}_{t-1})$ is the counterfactual state information if the history $H^{\pi_1}_{t-1}$ were observed. 
%Let $\bar{d}^{\pi}_t = \bar{d}^{\pi}_{t,\bar{S}_t}$ denote the action sequence under policy $\pi$ given the state sequence $\bar{S}_t$.
%$\bar{M}_{t}(\bar{d}^{\pi}_t) = \bar{M}_{t,\bar{S}_t}(\bar{d}^{\pi}_t)$

%Let $R_t(\bar{d}^{\pi_1}_t,\bar{M}_{t,\bar{d}^{\pi_2}_t})$ be the given $\bar{S}_t$,
We consider a three-way decomposition of TE$_t$ for target policy $\pi_e$ and control policy $\pi_0$, as follows.
\begin{equation}\label{eqn:PO_decomp}
\begin{alignedat}{4}
    & &&\textrm{TE}_t(\pi_e,\pi_0)\\
    &= &&\Mean^{\pi_e}\Big[R_t(\bar{d}^{\pi_e}_t,\bar{M}_{t}(\bar{d}^{\pi_e}_t))\Big] - \Mean^{\pi_0}\Big[R_t(\bar{d}^{\pi_0}_t,\bar{M}_{t}(\bar{d}^{\pi_0}_t))\Big],\\
    &= 
    &&\underbrace{\Mean^{\pi_e}\Big[R_t(\bar{d}^{\pi_e}_t,\bar{M}_{t}(\bar{d}^{\pi_e}_t))-R_t(\bar{d}^{\pi_0}_t,\bar{M}_{t}(\bar{d}^{\pi_e}_t))\Big]}_{\textrm{DE}_t(\pi_e,\pi_0)}\\
    & &&+\underbrace{\Mean^{\pi_e}\Big[R_t(\bar{d}^{\pi_0}_t,\bar{M}_{t}(\bar{d}^{\pi_e}_t))-R_t(\bar{d}^{\pi_0}_t,\bar{M}_{t}(\bar{d}^{\pi_0}_t))\Big]}_{\textrm{ME}_t(\pi_e,\pi_0)}\\
    & &&+\underbrace{\Mean^{\pi_e}\Big[R_t(\bar{d}^{\pi_0}_t,\bar{M}_{t}(\bar{d}^{\pi_0}_t))\Big]-\Mean^{\pi_0}\Big[R_t(\bar{d}^{\pi_0}_t,\bar{M}_{t}(\bar{d}^{\pi_0}_t))\Big]}_{\textrm{SE}_t(\pi_e,\pi_0)}.
\end{alignedat}
\end{equation}
Specifically, $\textrm{DE}_t(\pi_e,\pi_0)$ contrasts the impact of the random policy-induced action sequences $\bar{d}^{\pi_e}_t$ and $\bar{d}^{\pi_0}_t$ on the reward obtained at step $t$ when the mediator sequence and state sequence are set to the levels that would be seen if policy $\pi_e$ were followed; $\textrm{ME}_t(\pi_e,\pi_0)$ quantifies the difference in the effect of the mediator at levels $\bar{M}_{t,\bar{d}^{\pi_e}_t}$ and $\bar{M}_{t,\bar{d}^{\pi_0}_t}$ on the reward at step $t$, when the state sequence is set to the level under policy $\pi_e$ and the action sequence is set to $\bar{d}^{\pi_0}_t$ induced by policy $\pi_0$; and $\textrm{SE}_t(\pi_e,\pi_0)$ measures the difference in how the policy-induced state sequences $\bar{S}^{\pi_e}_t$ and $\bar{S}^{\pi_0}_t$ would affect the reward received at step $t$, when the $\pi_0$-induced action sequence is taken and the mediator is set to $\bar{M}_{t,\bar{d}^{\pi_0}_t}$.

\begin{remark} When $t=0$ and $S_0$ is used as covariate, we can show that $\textrm{ME}_0(\pi_e, \pi_0) = \textrm{ME}_0(\pi_e, \pi_0) + \textrm{SE}_0(\pi_e, \pi_0)$, which depicts the natural indirect effect (NIE). Considering comparing the effects of two fixed action sequences, $\bar{A}_t = \bar{a}_t^{*}$ and $\bar{A}_t = \bar{a}'_t$, we denote that $\textrm{DE}_t(\bar{a}_t^{*},\bar{a}'_t) = \Mean^{\bar{a}_t^{*}}[R_t(\bar{a}_t^{*},\bar{M}_{t}(\bar{a}_t^{*}))-R_t(\bar{a}'_t,\bar{M}_{t}(\bar{a}_t^{*}))]$ and $\textrm{ME}_t(\bar{a}_t^{*},\bar{a}'_t)$ and $\textrm{SE}_t(\bar{a}_t^{*},\bar{a}'_t)$ are analogously defined. When $t=0$, the direct effect ($\textrm{DE}_0(a_0^{*}, a'_0)$) and the indirect effect ($\textrm{ME}_0(a_0^{*}, a'_0)$ or $\textrm{ME}_0(a_0^{*}, a'_0)+\textrm{SE}_0(a_0^{*}, a'_0)$) represented above are equivalent to the natural direct effect (NDE) and NIE derived in \citet{pearl2022direct}. When $t>0$, the above definition is analogous to the definition of NIE and NDE discussed in \citet{vanderweele2017mediation}, in the context of time-varying treatments and mediators. However, when the state sequence (time-varying confounders in \citet{vanderweele2017mediation}) is not intervened appropriately, both the NIE and NDE in \citet{vanderweele2017mediation} include a part of the state effect.
\end{remark}

\section{Potential Outcome (Version 2)}

We first start with some notations. Define $\bar{a}_t = (a_0, \cdots, a_t) \in \mathcal{A}_t$. Let $\bar{S}^{*}_t(\bar{a}_t) = \{S_0, S^{*}_1(a_0),\cdots, S^{*}_t(\bar{a}_{t-1})\}$, where $S^{*}_t(\bar{a}_{t-1})$ denotes the potential state at time $t$ under the treatment sequence $\bar{a}_{t-1}$. For simplicity, let $\bar{s}_t = (s_0,\cdots,s_t) \in \mathcal{S}_t$ be a fixed state sequence.  Conditional on $\bar{s}_t$, let $\bar{M}^{*}_t(\bar{a}_t) = \{M^{*}_0(a_0),\cdots, M^{*}_t(\bar{a}_{t})\}$, where $M^{*}_t(\bar{a}_{t})$ is the potential mediator and at time $t$ under the treatment sequence $\bar{a}_{t}$. Similarly, conditional on $\bar{s}_t$, let $R^{*}_t(\bar{a}^{1}_t, \bar{M}^{*}_t(\bar{a}^{2}_t))$ denote the potential reward that would be observed at time $t$ if under the treatment sequence $\bar{a}^{1}_{t-1}$ with the mediator sequence being set to $\bar{M}^{*}_t(\bar{a}^{2}_t)$, where $\bar{a}^{1}_t$ and $\bar{a}^{2}_t$ can be two different action sequences. 

For any policy $\pi$, denote $\{d_t^{\pi}(\cdot)\}_{t>0}$ a sequence of independent, $\mathcal{A}$-valued stochastic process indexed by $\mathcal{S}_t$ such that $P\{d_t^{\pi}(s_{t}) = a_t\} = \pi(a_t|s_t)$. Then the potential state at time $t$ under policy $\pi$ is
\begin{equation}
    S_t^{*}(\pi) = \sum_{\bar{a}_{t-1}\in\mathcal{A}_{t-1}}S^{*}_t(\bar{a}_{t-1})\prod_{j=0}^{t-1}1[d_{j}^{\pi}\{S^{*}_j(\bar{a}_{j-1})\}=a_j],
\end{equation}
where $S^{*}_0(\bar{a}_{-1})= S_0$. Conditional on $\bar{s}_t$, the potential mediator under policy $\pi$ at time $t$ is 
\begin{equation}
    M^{*}_t(\pi) = \sum_{\bar{a}_{t}\in\mathcal{A}_{t}}M^{*}_t(\bar{a}_{t})\prod_{j=0}^{t}1[d_{j}^{\pi}\{s_j\}=a_j],
\end{equation} and the potential reward under policy $\pi_{1}$ with mediator sequence being set to $M^{*}_t(\pi_{2})$ is
\begin{equation}
    R^{*}_t(\pi_{1}, M^{*}_t(\pi_{2})) = \sum_{\bar{a}_{t}\in\mathcal{A}_{t}}R^{*}_t(\bar{a}_{t}, M^{*}_t(\pi_{2}))\prod_{j=0}^{t}1[d_{j}^{\pi_{1}}\{s_j\}=a_j].
\end{equation}

To evaluate the treatment effect, we consider a three-way decomposition of TE$_t$ for target policy $\pi_e$ and control policy $\pi_0$, as follows.
\begin{equation}\label{eqn:PO_decomp}
\begin{alignedat}{4}
    & &&\textrm{TE}_t(\pi_e,\pi_0)\\
    &= &&\Mean\left\{\Mean\left[R^{*}_t(\pi_e,\bar{M}^{*}_{t}(\pi_e))\;\middle|\;\bar{S}_t^{*}(\pi_e)\right]\right\} -\Mean\left\{\Mean\left[R^{*}_t(\pi_0,\bar{M}^{*}_{t}(\pi_0))\;\middle|\;\bar{S}_t^{*}(\pi_0)\right]\right\},\\
    &= &&\underbrace{\Mean\left\{\Mean\left[R^{*}_t(\pi_e,\bar{M}^{*}_{t}(\pi_e))-R^{*}_t(\pi_0,\bar{M}^{*}_{t}(\pi_e))\;\middle|\;\bar{S}_t^{*}(\pi_e)\right]\right\}}_{\textrm{DE}_t(\pi_e,\pi_0)}\\
    & &&+\underbrace{\Mean\left\{\Mean\left[R^{*}_t(\pi_0,\bar{M}^{*}_{t}(\pi_e))-R^{*}_t(\pi_0,\bar{M}^{*}_{t}(\pi_0))\;\middle|\;\bar{S}_t^{*}(\pi_e)\right]\right\}}_{\textrm{ME}_t(\pi_e,\pi_0)}\\
    & &&+\underbrace{\Mean\left\{\Mean\left[R^{*}_t(\pi_0,\bar{M}^{*}_{t}(\pi_0))\;\middle|\;\bar{S}_t^{*}(\pi_e)\right]\right\}-\Mean\left\{\Mean\left[R^{*}_t(\pi_0,\bar{M}^{*}_{t}(\pi_0))\;\middle|\;\bar{S}_t^{*}(\pi_0)\right]\right\}}_{\textrm{SE}_t(\pi_e,\pi_0)}.
\end{alignedat}
\end{equation}
Specifically, $\textrm{DE}_t(\pi_e,\pi_0)$ contrasts the impact of the $\pi_e$-induced action sequence and $\pi_0$-induced action sequence on the reward obtained at step $t$ when the mediator sequence and state sequence are set to the levels that would be seen if policy $\pi_e$ were followed; $\textrm{ME}_t(\pi_e,\pi_0)$ quantifies the difference in the effect of the mediator at levels $\bar{M}_t^{*}(\pi_e)$ and $\bar{M}_t^{*}(\pi_0)$ on the reward at step $t$, when the state sequence is set to the level under $\pi_e$ with an action sequence induced by $\pi_0$; and $\textrm{SE}_t(\pi_e,\pi_0)$ measures the difference in how the policy-induced state sequences $\bar{S}^{*}_t(\pi_e)$ and $\bar{S}^{*}_t(\pi_0)$ would affect the reward received at step $t$, when the $\pi_0$-induced action sequence is taken and the mediator is set to $\bar{M}^{*}_{t}(\pi_0)$.

\begin{remark} When $t=0$ and $S_0$ is used as covariate, we can show that $\textrm{SE}_0(\pi_e, \pi_0) = 0$. Considering comparing the effects of two fixed action sequences, $\bar{a}_t^{1}$ and $\bar{a}^{2}_t$, we denote that $\textrm{DE}_t(\bar{a}_t^{1},\bar{a}_t^{2}) = \Mean\left\{\Mean\left[R^{*}_t(\bar{a}_t^{1},\bar{M}^{*}_{t}(\bar{a}_t^{1}))-R^{*}_t(\bar{a}_t^{2},\bar{M}^{*}_{t}(\bar{a}_t^{1}))\;\middle|\;\bar{S}_t^{*}(\bar{a}_t^{1})\right]\right\}$ and analogously define $\textrm{ME}_t(\bar{a}_t^{1},\bar{a}^{2}_t)$ and $\textrm{SE}_t(\bar{a}_t^{1},\bar{a}^{2}_t)$. When $t=0$, the direct effect, $\textrm{DE}_0(a_0^{1}, a_0^{2})$ and the indirect effect $\textrm{ME}_0(a_0^{1}, a_0^{2})$ are equivalent to the natural direct effect (NDE) and natural indirect effect (NIE) derived in \citet{pearl2022direct}. When $t>0$, the above definition is analogous to the definition of NIE and NDE discussed in \citet{vanderweele2017mediation}, in the context of time-varying treatments and mediators. However, when the state sequence (referred as time-varying confounders in \citet{vanderweele2017mediation}) is not intervened appropriately, both the NIE and NDE in \citet{vanderweele2017mediation} include a part of the state effect.
\end{remark}

\section{Potential Outcome (Version 3)}
For any policy $\pi$, denote $\{d_t^{\pi}(\cdot)\}_{t>0}$ a sequence of independent, $\mathcal{A}$-valued stochastic process indexed by $\mathcal{S}_t$ such that $P\{d_t^{\pi}(s_{t}) = a_t\} = \pi(a_t|s_t)$. Then the potential state at time $t$ under policy $\pi$ is
\begin{equation}
    S_t^{*}(\pi) = \sum_{\bar{a}_{t-1}\in\mathcal{A}_{t-1}}S^{*}_t(\bar{a}_{t-1},\bar{M}^{*}_{t-1}(\bar{a}_{t-1})|\bar{S}^{*}_{t-1}(\pi))\prod_{j=0}^{t-1}1[d_{j}^{\pi}\{S^{*}_j(\bar{a}_{j-1},\bar{M}^{*}_{t-1}(\bar{a}_{j-1})|\bar{S}^{*}_{t-1}(\pi))\}=a_j],
\end{equation}
where $S^{*}_0(\bar{a}_{-1})= S_0$ and the conditional potential mediator is defined as 
\begin{equation}
    M^{*}_t(\pi)|\bar{S}_t^{*}(\pi') = \sum_{\bar{a}_{t}\in\mathcal{A}_{t}}M^{*}_t(\bar{a}_{t})\prod_{j=0}^{t}1[d_{j}^{\pi}\{S^{*}_{j}(\pi')\}=a_j],
\end{equation} and the potential reward under policy $\pi_{1}$ with mediator sequence being set to $\bar{M}^{*}_t(\pi_{2},\pi_{3})$ is
\begin{equation}
    R^{*}_t(\pi_{1}, \bar{M}^{*}_t(\pi_{2}))| \bar{S}_t^{*}(\pi')= \sum_{\bar{a}_{t}\in\mathcal{A}_{t}}R^{*}_t(\bar{a}_{t}, \bar{M}^{*}_t(\pi_{2})|\bar{S}_t^{*}(\pi'))\prod_{j=0}^{t}1[d_{j}^{\pi_{1}}\{S^{*}_j(\pi')\}=a_j].
\end{equation}

To evaluate the treatment effect, we consider a three-way decomposition of TE$_t$ for target policy $\pi_e$ and control policy $\pi_0$, as follows.
\begin{equation}\label{eqn:PO_decomp}
\begin{alignedat}{4}
    & &&\textrm{TE}_t(\pi_e,\pi_0)\\
    &= &&\Mean\left\{\Mean\left[R^{*}_t(\pi_e,\bar{M}^{*}_{t}(\pi_e))\;\middle|\;\bar{S}_t^{*}(\pi_e)\right]\right\} -\Mean\left\{\Mean\left[R^{*}_t(\pi_0,\bar{M}^{*}_{t}(\pi_0))\;\middle|\;\bar{S}_t^{*}(\pi_0)\right]\right\},\\
    &= &&\underbrace{\Mean\left\{\Mean\left[R^{*}_t(\pi_e,\bar{M}^{*}_{t}(\pi_e))-R^{*}_t(\pi_0,\bar{M}^{*}_{t}(\pi_e))\;\middle|\;\bar{S}_t^{*}(\pi_e)\right]\right\}}_{\textrm{DE}_t(\pi_e,\pi_0)}\\
    & &&+\underbrace{\Mean\left\{\Mean\left[R^{*}_t(\pi_0,\bar{M}^{*}_{t}(\pi_e))-R^{*}_t(\pi_0,\bar{M}^{*}_{t}(\pi_0))\;\middle|\;\bar{S}_t^{*}(\pi_e)\right]\right\}}_{\textrm{ME}_t(\pi_e,\pi_0)}\\
    & &&+\underbrace{\Mean\left\{\Mean\left[R^{*}_t(\pi_0,\bar{M}^{*}_{t}(\pi_0))\;\middle|\;\bar{S}_t^{*}(\pi_e)\right]\right\}-\Mean\left\{\Mean\left[R^{*}_t(\pi_0,\bar{M}^{*}_{t}(\pi_0))\;\middle|\;\bar{S}_t^{*}(\pi_0)\right]\right\}}_{\textrm{SE}_t(\pi_e,\pi_0)}.
\end{alignedat}
\end{equation}

\section{Potential Outcome (Version 4)}
For any policy $\pi$, denote $\{d_t^{\pi}(\cdot)\}_{t>0}$ a sequence of independent, $\mathcal{A}$-valued stochastic process indexed by $\mathcal{S}_t$ such that $P\{d_t^{\pi}(s_{t}) = a_t\} = \pi(a_t|s_t)$. Then the potential state at time $t$ under policy $\pi$ is
\begin{equation}
    S_t^{*}(\pi) = \sum_{\bar{a}_{t-1}\in\mathcal{A}_{t-1}}S^{*}_t(\bar{a}_{t-1},\bar{M}^{*}_{t-1}(\bar{a}_{t-1})|\bar{S}^{*}_{t-1}(\pi))\prod_{j=0}^{t-1}1[d_{j}^{\pi}\{S^{*}_j(\bar{a}_{j-1},\bar{M}^{*}_{t-1}(\bar{a}_{j-1})|\bar{S}^{*}_{t-1}(\pi))\}=a_j],
\end{equation}
where $S^{*}_0(\bar{a}_{-1})= S_0$ and the potential mediator conditional on the state sequence is defined as 
\begin{equation}
    M^{*}_t(\pi)|S_t^{*}(\pi') = \sum_{a_{t}\in\mathcal{A}}M^{*}_t(a_{t})1[d_{j}^{\pi}\{S^{*}_{t}(\pi')\}=a_t],
\end{equation} and the potential reward under policy $\pi_{1}$ with mediator sequence being set to $\bar{M}^{*}_t(\pi_{2},\pi_{3})$ is
\begin{equation}
    R^{*}_t(\pi_{1}, M^{*}_t(\pi_{2}))| S_t^{*}(\pi')= \sum_{a_{t}\in\mathcal{A}}R^{*}_t(a_{t}, M^{*}_t(\pi_{2})|S_t^{*}(\pi'))1[d_{t}^{\pi_{1}}\{S^{*}_t(\pi')\}=a_t].
\end{equation}

To evaluate the treatment effect, we consider a three-way decomposition of TE$_t$ for target policy $\pi_e$ and control policy $\pi_0$, as follows.
\begin{equation}\label{eqn:PO_decomp}
\begin{alignedat}{4}
    & &&\textrm{TE}_t(\pi_e,\pi_0)\\
    &= &&\Mean\left\{\Mean\left[R^{*}_t(\pi_e,M^{*}_{t}(\pi_e))\;\middle|\;S_t^{*}(\pi_e)\right]\right\} -\Mean\left\{\Mean\left[R^{*}_t(\pi_0,M^{*}_{t}(\pi_0))\;\middle|\;S_t^{*}(\pi_0)\right]\right\},\\
    &= &&\underbrace{\Mean\left\{\Mean\left[R^{*}_t(\pi_e,M^{*}_{t}(\pi_e))-R^{*}_t(\pi_0,M^{*}_{t}(\pi_e))\;\middle|\;S_t^{*}(\pi_e)\right]\right\}}_{\textrm{DE}_t(\pi_e,\pi_0)}\\
    & &&+\underbrace{\Mean\left\{\Mean\left[R^{*}_t(\pi_0,M^{*}_{t}(\pi_e))-R^{*}_t(\pi_0,M^{*}_{t}(\pi_0))\;\middle|\;S_t^{*}(\pi_e)\right]\right\}}_{\textrm{ME}_t(\pi_e,\pi_0)}\\
    & &&+\underbrace{\Mean\left\{\Mean\left[R^{*}_t(\pi_0,M^{*}_{t}(\pi_0))\;\middle|\;S_t^{*}(\pi_e)\right]\right\}-\Mean\left\{\Mean\left[R^{*}_t(\pi_0,M^{*}_{t}(\pi_0))\;\middle|\;S_t^{*}(\pi_0)\right]\right\}}_{\textrm{SE}_t(\pi_e,\pi_0)}.
\end{alignedat}
\end{equation}
