# Supplementary material for: A Reinforcement Learning Framework for Dynamic Mediation Analysis
Source: arXiv:2301.13348 source file (2023-09-03)
Supplement: Supplementary file 3 [file SE_decomp.tex]

\section{Decomposition of $SE(\pi_e,\pi_0)$}
We further decompose the $SE(\pi_e,\pi_0)$ into the delayed mediator effect $D-ME(\pi_e,\pi_0)$ and the delayed direct effect $D-DE(\pi_e,\pi_0)$.
\begin{align*}
&\Mean\left[R^{*}_t(\pi_{e,0}^{t},\bar{M}^{*}_{t}(\pi_{e,0}^{t})\right]-\Mean\left[R^{*}_t(\pi_0,\bar{M}^{*}_{t}(\pi_0))\right] \\
=&\underbrace{\Mean\left[R^{*}_t(\pi_{e,0}^{t},\bar{M}^{*}_{t}(\pi_{e,0}^{t})\right] - \Mean\left[R^{*}_t(\pi_{0},\bar{G}^{*}_{t}(\pi_{e,0}^{t}))\right]}_{PDE(\pi_e,\pi_0)} + \underbrace{\Mean\left[R^{*}_t(\pi_{0},\bar{G}^{*}_{t}(\pi_{e,0}^{t}))\right] -
\Mean\left[R^{*}_t(\pi_0,\bar{M}^{*}_{t}(\pi_0))\right]}_{PME(\pi_e,\pi_0)},
\end{align*} where the identification function of $R^{*}_t(\pi_{0},\bar{G}^{*}_{t}(\pi_{e,0}^{t}))$ is
\begin{multline*}
    \sum_{\tau_t,\tau^*_t}r_t p(s_{t+1},r_t|s_t,a_t,m_t)p(m_t|s_t,a_t)\pi_0(a_t|s_t)\prod_{j=0}^{t-1}p(s_{j+1},r_j|s_j,a_j,m_j)\pi_0(a_j|s_j)\\
    \prod_{l=1}^{t-1}p(m_l|a^*_l,s^*_l)\pi_e(a^*_l|s^*_l)p(s^*_l,r^*_{l-1}|s^*_{l-1},a^*_{l-1},m_{l-1}) \times p(m_0|a^*_0,s_0)\pi_e(a^*_0|s_0)\nu(s_0).
\end{multline*} It can be rewritten as
\begin{multline*}
    \sum_{\tau_t,\tau^*_t}r_t p(s_{t+1},r_t|s_t,a_t,m_t)p(m_t|s_t,a_t)\pi_0(a_t|s_t)\prod_{j=0}^{t-1}p(s_{j+1},r_j|s_j,a_j,m_j)\pi_0(a_j|s_j)
    p(s^*_{j+1},r^*_j|s^*_j,a^*_j,m_j)\pi_e(a^*_j|s^*_j)
    p(m_j|s^*_j,a^*_j)\\
    \nu(s_0),
\end{multline*}where $s^*_0 = s_0$.
Equivalently,
\begin{multline*}
    \sum_{\tau_t,\tau^*_t}r_t p_{\theta_0}(s_{t+1},r_t|s_t,a_t,m_t)p_{\theta_0}(m_t|s_t,a_t)\pi_0(a_t|s_t)\prod_{j=0}^{t-1}p_{\theta_0}(s_{j+1},r_j|s_j,a_j,m_j)\pi_0(a_j|s_j)
    p_{\theta_0}^{\pi_e}(s^*_{j+1},r^*_j,m_j,a^*_j|s^*_j)\nu_{\theta_0}(s_0).
\end{multline*}
Taking derivative,
\begin{multline*}
    \lim_{T\to\infty}\frac{1}{T}\sum_{t=0}^{T-1}\sum_{\tau_t,\tau^*_t}r_t p_{\theta_0}(s_{t+1},r_t|s_t,a_t,m_t)p_{\theta_0}(m_t|s_t,a_t)\pi_0(a_t|s_t)\prod_{j=0}^{t-1}p_{\theta_0}(s_{j+1},r_j|s_j,a_j,m_j)\pi_0(a_j|s_j)
    p_{\theta_0}^{\pi_e}(s^*_{j+1},r^*_j,m_j,a^*_j|s^*_j)\\
    \Big\{ \sum_{j=0}^{t-1}\triangledown_{\theta}\log p_{\theta_0}(s_{j+1},r_j|s_j,a_j,m_j) + \triangledown_{\theta}\log p_{\theta_0}(s_{t+1},r_{t},m_t|s_t,a_t)+\sum_{j=0}^{t-1}\triangledown_{\theta}\log p_{\theta_0}^{\pi_e}(s^*_{j+1},r^*_j,m_j,a^*_j|s^*_j)\Big\}\nu_{\theta_0}(s_0),
\end{multline*}where $s^*_0 = s_0$.

We first focus on the part I:
\begin{multline*}
    \lim_{T\to\infty}\frac{1}{T}\sum_{t=0}^{T-1}\sum_{\tau_t,\tau^*_t}r_t p_{\theta_0}(s_{t+1},r_t|s_t,a_t,m_t)p_{\theta_0}(m_t|s_t,a_t)\pi_0(a_t|s_t)\prod_{j=0}^{t-1}p_{\theta_0}(s_{j+1},r_j|s_j,a_j,m_j)\pi_0(a_j|s_j)
    p_{\theta_0}^{\pi_e}(s^*_{j+1},r^*_j,m_j,a^*_j|s^*_j)\\
    \sum_{j=0}^{t}\triangledown_{\theta}\log p_{\theta_0}(s_{j+1},r_j|s_j,a_j,m_j)\nu_{\theta_0}(s_0),
\end{multline*}where $s^*_0 = s_0$
Since $\star$, the above function can be rewritten as
\begin{multline*}
    \lim_{T\to\infty}\frac{1}{T}\sum_{j=0}^{T-1}\sum_{\tau_t,\tau^*_t}[r_t-\Mean_{m^*}r_{\theta_0}(s_j,a_j,m^*)] p_{\theta_0}(s_{j+1},r_j, m_j|s_j,a_j)\pi_0(a_j|s_j)\\
    \prod_{k=0}^{j-1}p_{\theta_0}(s_{k+1},r_k|s_k,a_k,m_k)\pi_0(a_k|s_k)
    p_{\theta_0}^{\pi_e}(s^*_{k+1},r^*_k,m_k,a^*_k|s^*_k)\nu_{\theta_0}(s_0) \\
    \triangledown_{\theta}\log p_{\theta_0}(s_{j+1},r_j|s_j,a_j,m_j).
\end{multline*}
Further, since 
\begin{multline*}
    \sum_{s_0}\prod_{k=0}^{j}p_{\theta_0}(s_{k+1},r_k|s_k,a_k,m_k)\pi_0(a_k|s_k)
    p_{\theta_0}^{\pi_e}(s^*_{k+1},r^*_k,m_k,a^*_k|s^*_k)\nu_{\theta_0}(s_0) = \\
    p_{\theta_0}(s_{j+1},r_j|s_j,a_j,m_j)\pi_0(a_j|s_j)p^{G}(s_j)p_{\theta_0}^{\pi_e}(s^*_{j+1},r^*_j,m_j,a^*_j|s^*_j)p^{\pi_e}(s^*_j),
\end{multline*} we have that
\begin{multline*}
    \lim_{T\to\infty}\frac{1}{T}\sum_{j=0}^{T-1}\sum_{\tau_t,\tau^*_t}[r_t-\Mean_{m^*}r_{\theta_0}(s_j,a_j,m^*)] p_{\theta_0}(s_{j+1},r_j, m_j|s_j,a_j)\pi_0(a_j|s_j)p^{G}(s_j) \\
    \triangledown_{\theta}\log p_{\theta_0}(s_{j+1},r_j|s_j,a_j,m_j).
\end{multline*}

\begin{enumerate}
    \item Novelty:  mediation effect analysis on infinite horizon
    \item Motivation: total effect = IDE+IME+DDE+DME, 
        \begin{itemize}
            \item \textbf{Q1 (interventional):} whether mediation effect dominant the total effect---whether intervene on mediators or not
            \item \textbf{Q2 (understanding):} whether the proximal effect dominant the immediate effect---determine whether a policy depends on continuous long-term treatment
            (i.e., will such an interpretation of the delayed effect have conflict with the conditional independence of the MDP)
        \end{itemize}
    \item real data analysis: 
    \begin{itemize}
        \item \textbf{Q1:} get the ATE of $a=1$ compared to $a=0$, to get a clearer understanding about the weights of different effect components.
        \item \textbf{Q2:} take the behavior policy and estimated optimal policy as examples.
    \end{itemize}
\end{enumerate}
