# Supplementary material for: A Reinforcement Learning Framework for Dynamic Mediation Analysis
Source: arXiv:2301.13348 source file (2023-09-03)
Supplement: Supplementary file 4 [file Plan.tex]

\newpage
\section{Project Tasks}
\begin{itemize}
\item Numerical Experiments
\begin{itemize}
    \item toy example (completed)
    \item code for the simulation (reviewed Liao's R code)
    \item conduct simulation
    \item real experimentation
\end{itemize}
\item Theoretical Results
\begin{itemize}
    \item estimator derivation (completed)
    \item theorem proof (robustness, need to be more formal)
\end{itemize}
\end{itemize}
